# Supplementary material for: Hybrid Eigensolvers for Nuclear Configuration Interaction Calculations
Source: arXiv:2305.15552 source file (2023-05-24)
Supplement: Supplementary file 1 [file appendix.tex]

\clearpage
\section{APPENDIX}

\begin{figure}[htbp]
\centering
\includegraphics[scale=0.4]{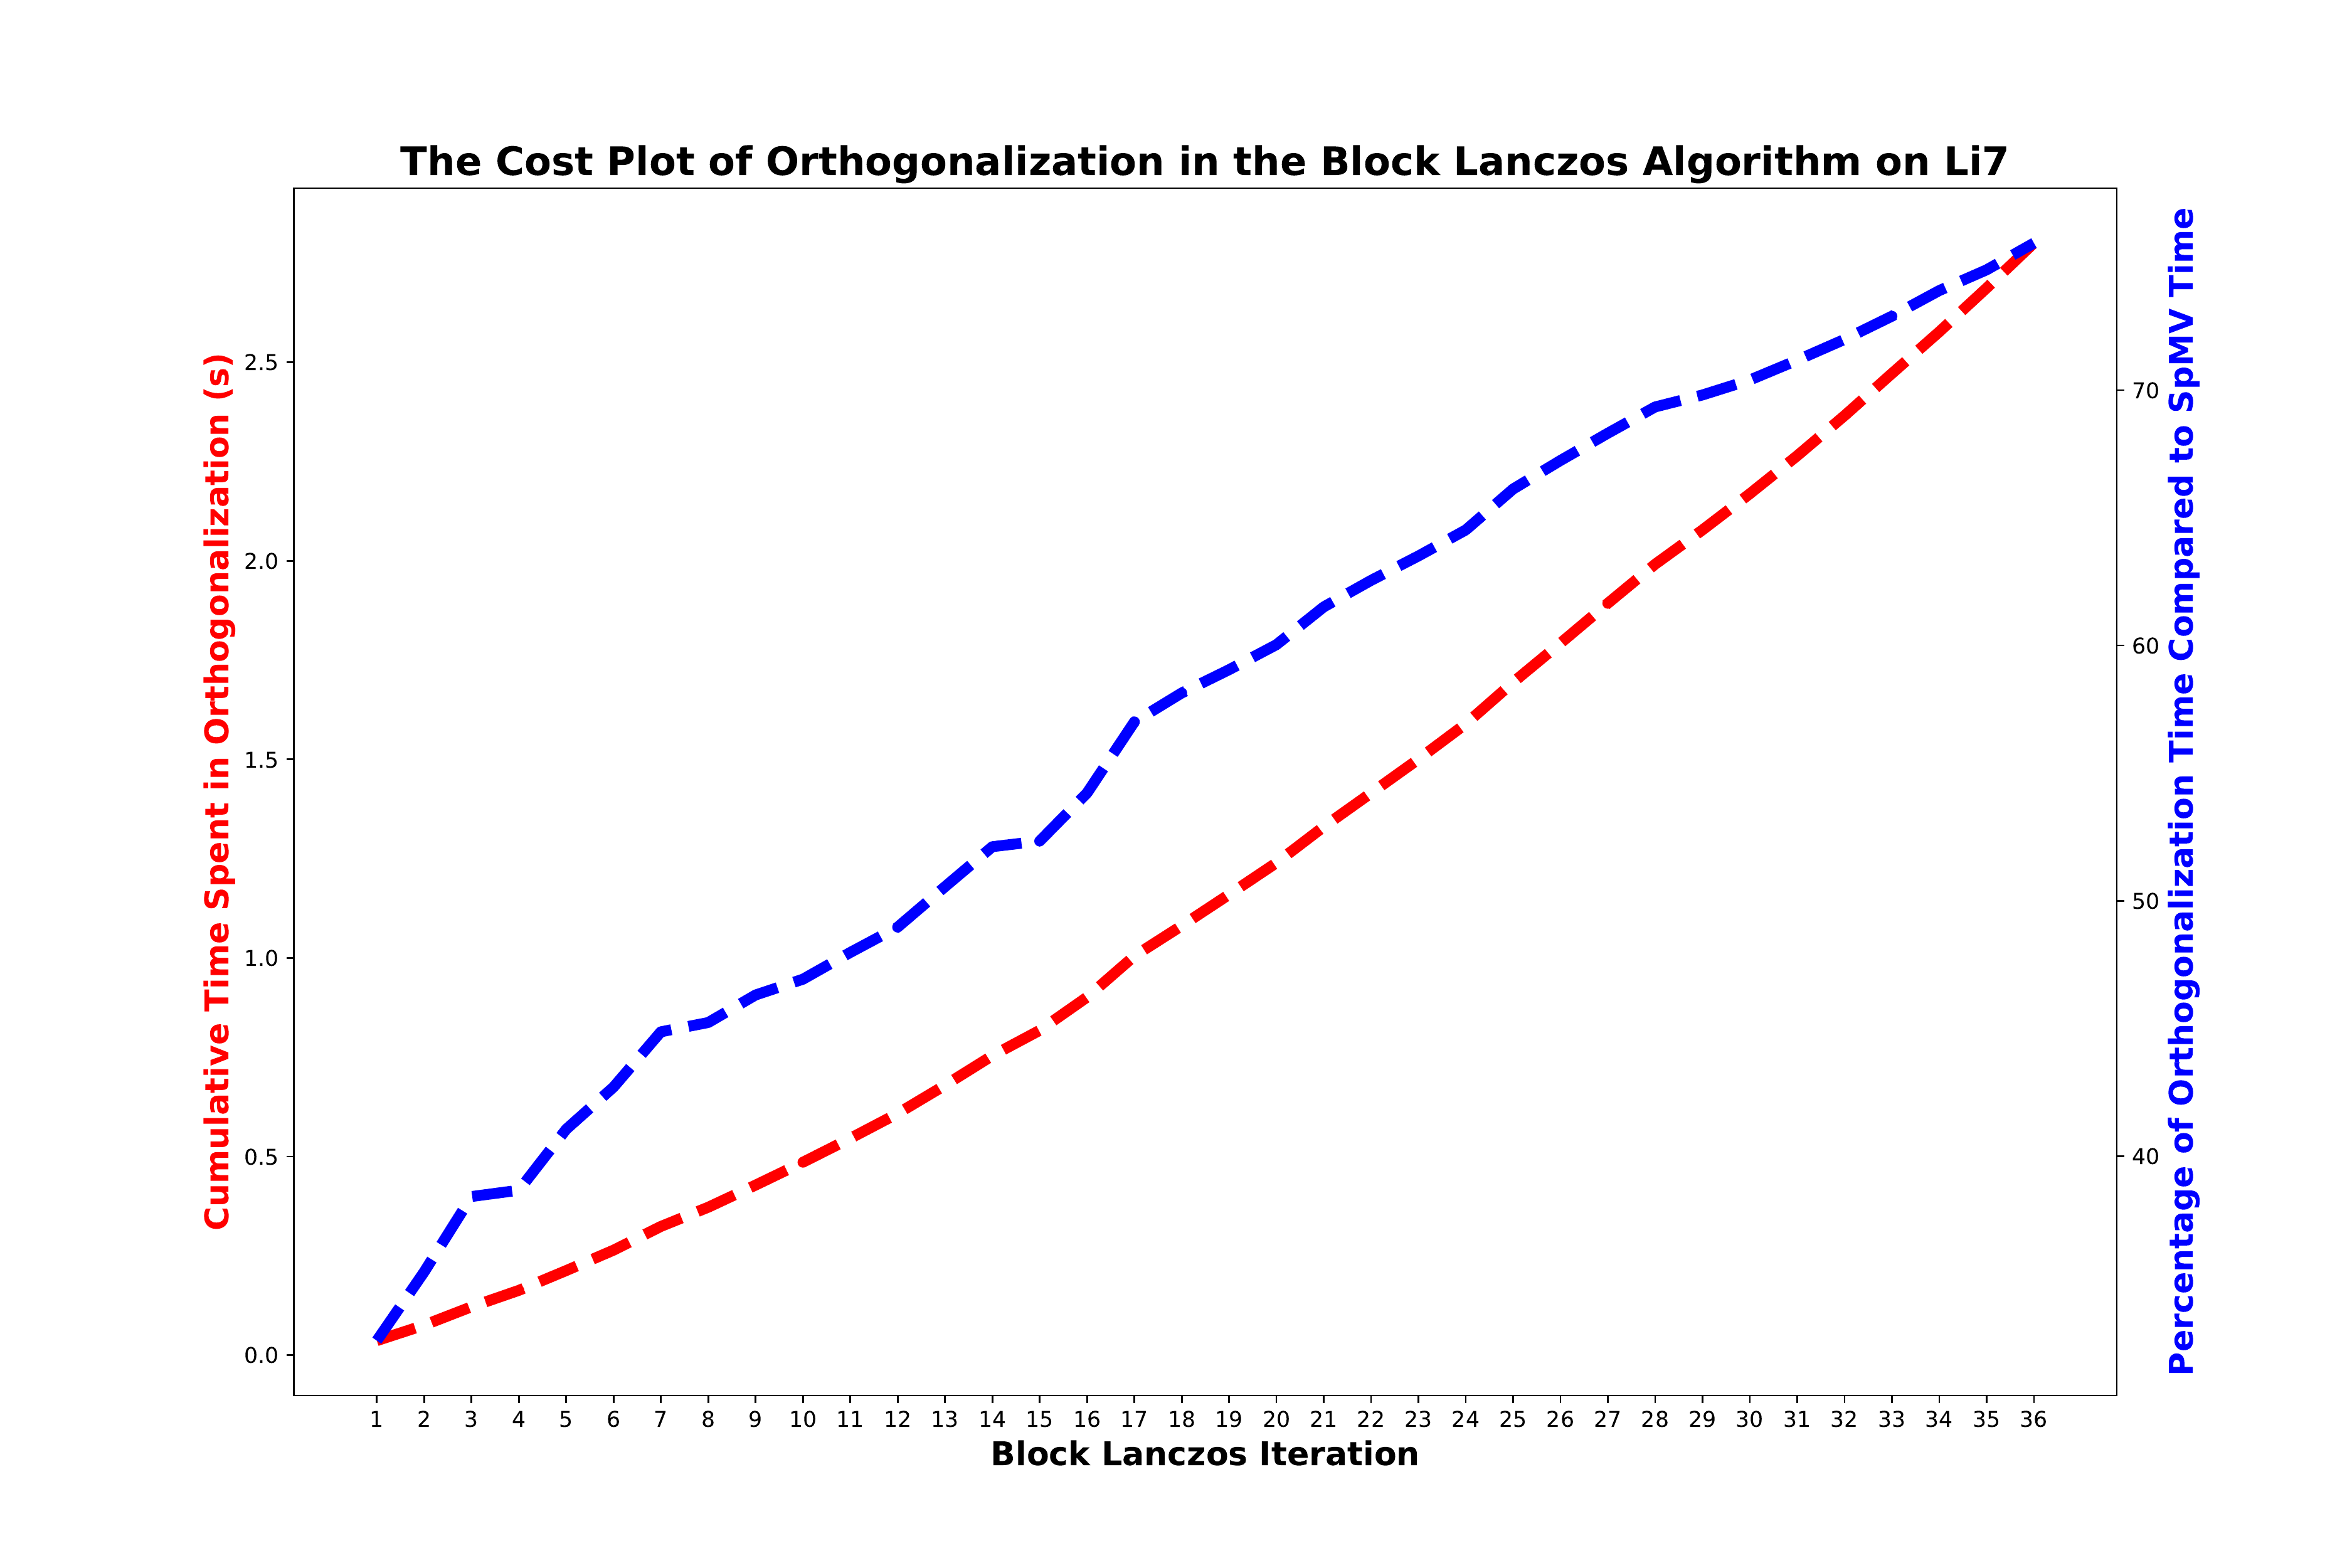}
\caption{The Cost Plot of Orthogonalization in the Block Lanczos Algorithm on Li7}
\label{fig:Li7BlockLanOrthCost}
\end{figure}

\begin{figure}[htbp]
\centering
\includegraphics[scale=0.6]{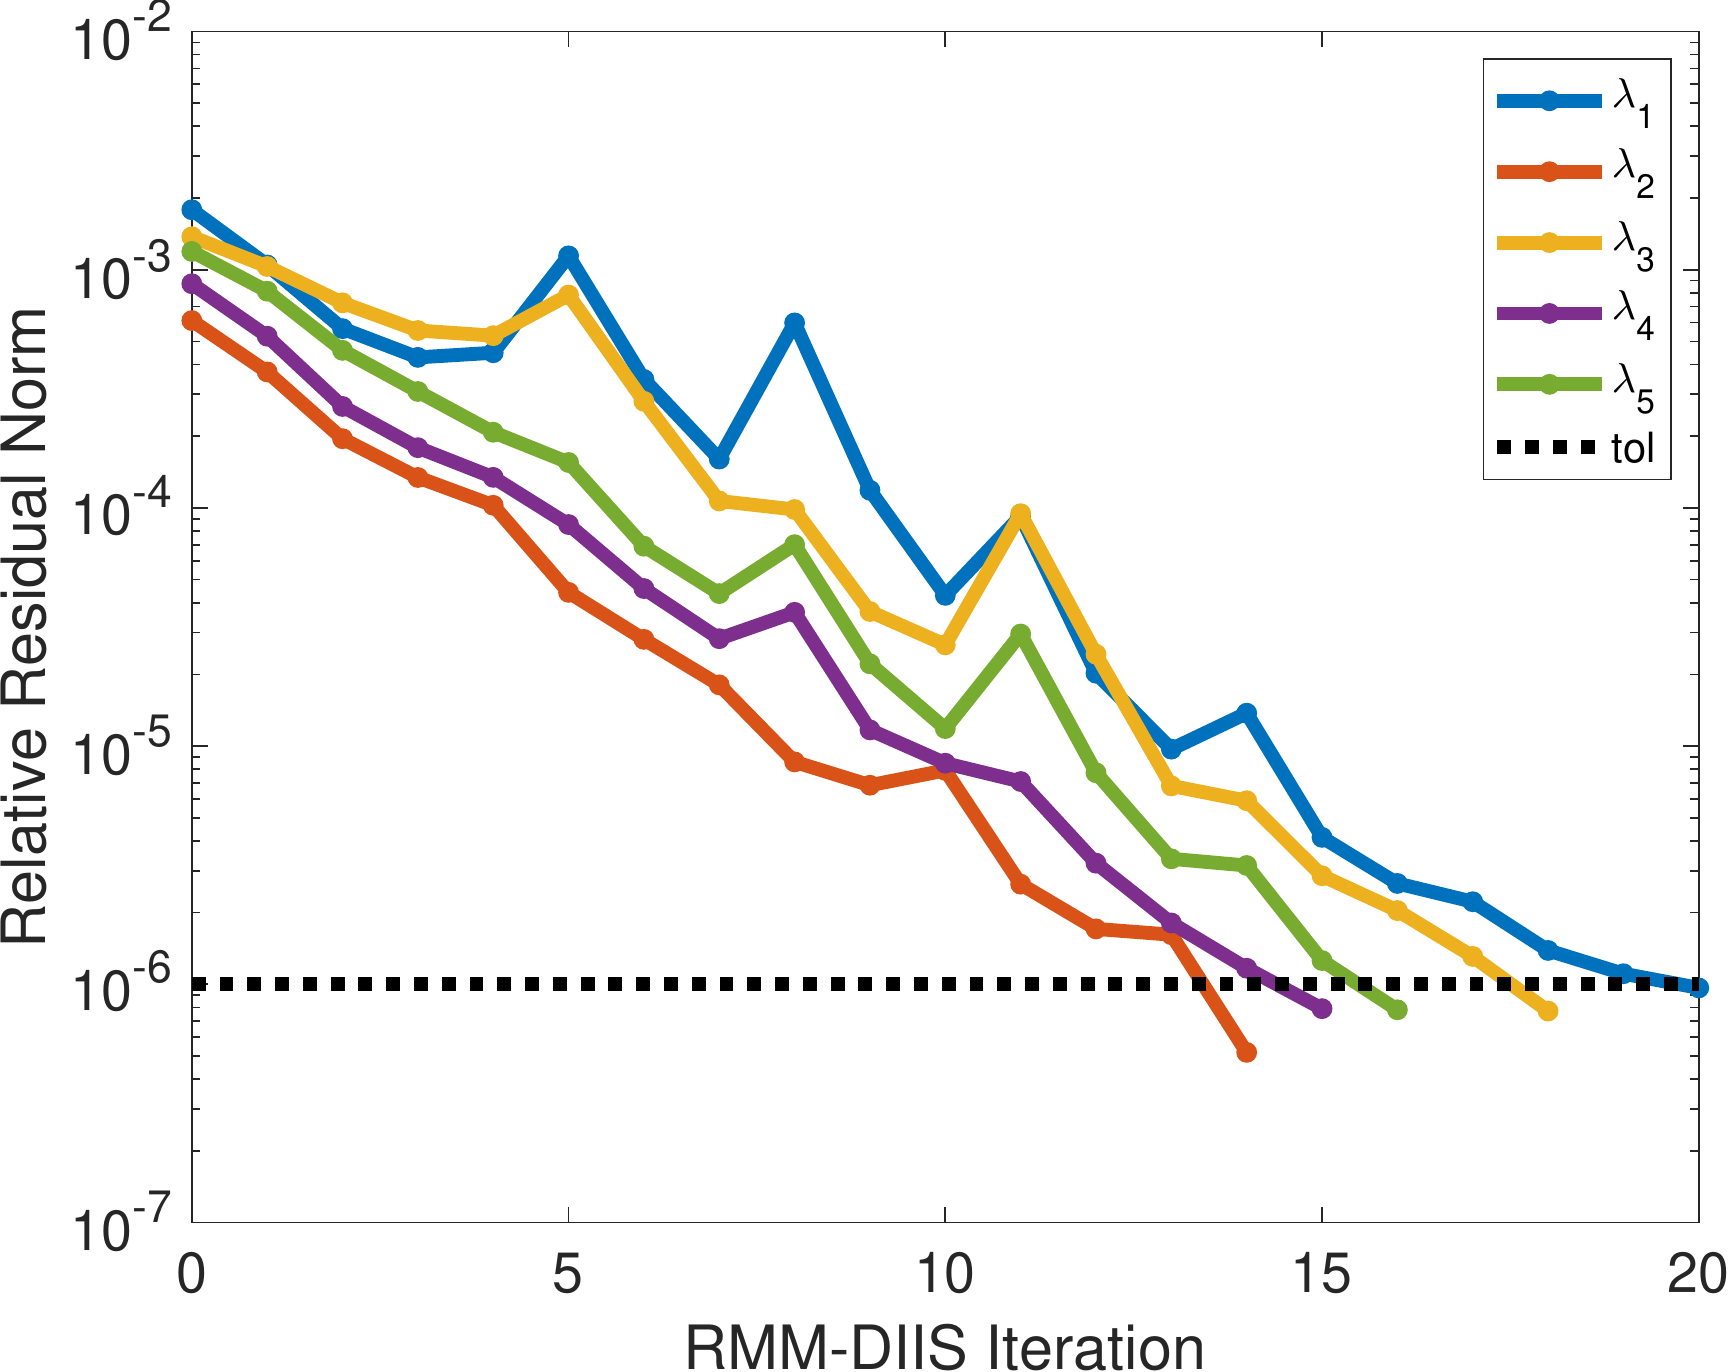}
\caption{The convergence of the lowest 5 eigenvalues of the Li6 Hamiltonian in the RMM-DIIS algorithm after 10 iterations of block Lanczos.}
\label{fig:Li6ConvBlockLanRMMDIIS}
\end{figure}
